# Supplementary material for: Improving Compound Activity Classification via Deep Transfer and Representation Learning
Source: arXiv:2111.07439 source file (2022-03-09)
Supplement: Supplementary file 1 [file supp_param_study_best_tasks_aada_dmpna_LG.tex]

\begin{figure*}[h!]
    \centering
    \begin{subfigure}{0.32\textwidth}
        \centering
        \includegraphics[width=\textwidth]{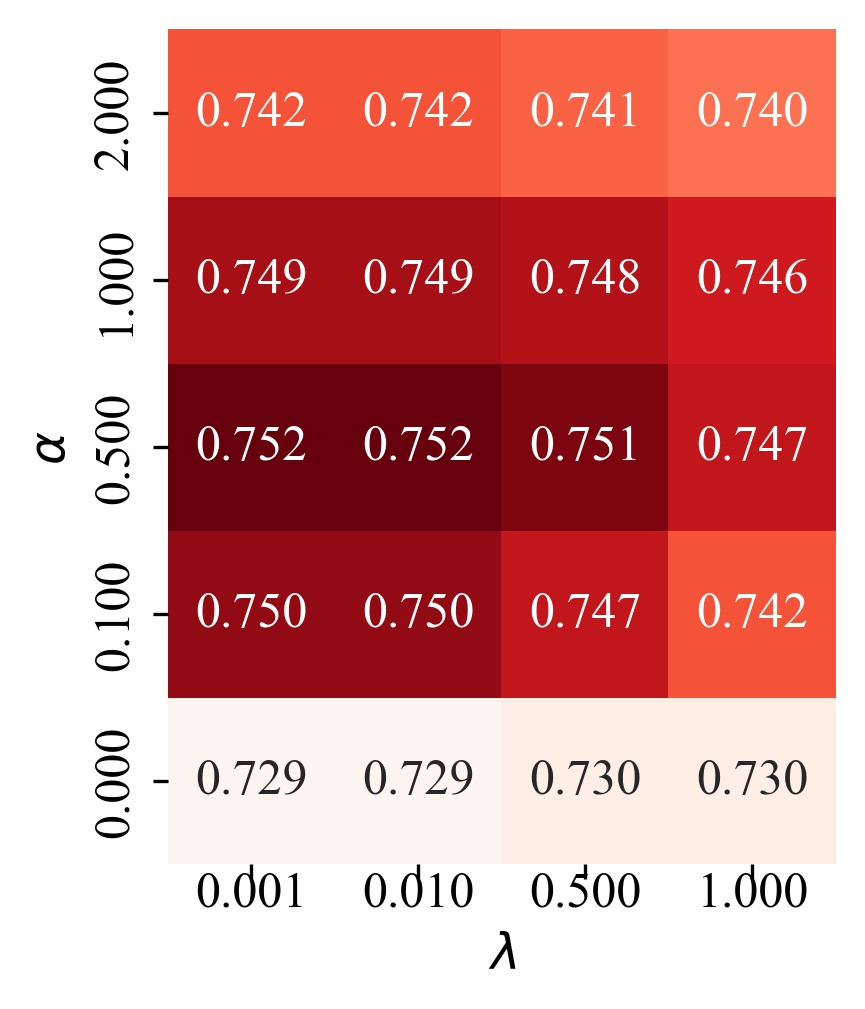}
        \caption{\prauc}
    \end{subfigure}
     ~ 
    \begin{subfigure}{0.32\textwidth}
        \centering
        \includegraphics[width=\textwidth]{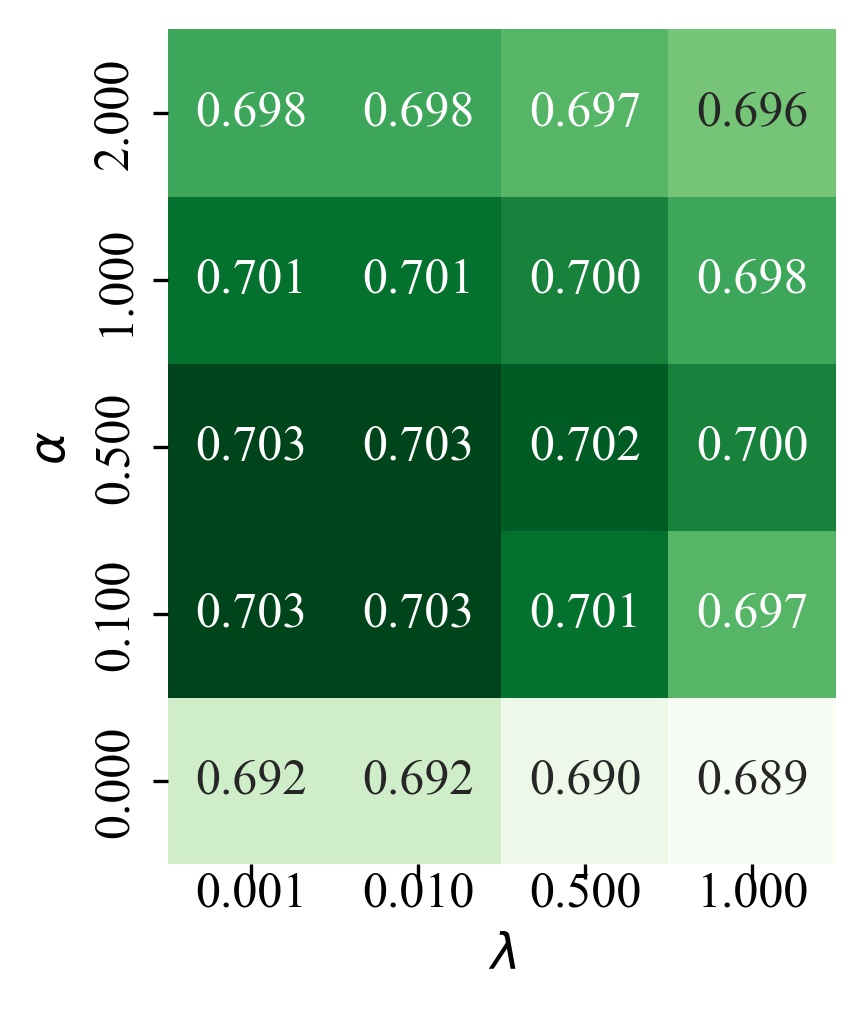}
        \caption{\precision}
    \end{subfigure}
     ~
    \begin{subfigure}{0.32\textwidth}
        \centering
        \includegraphics[width=\textwidth]{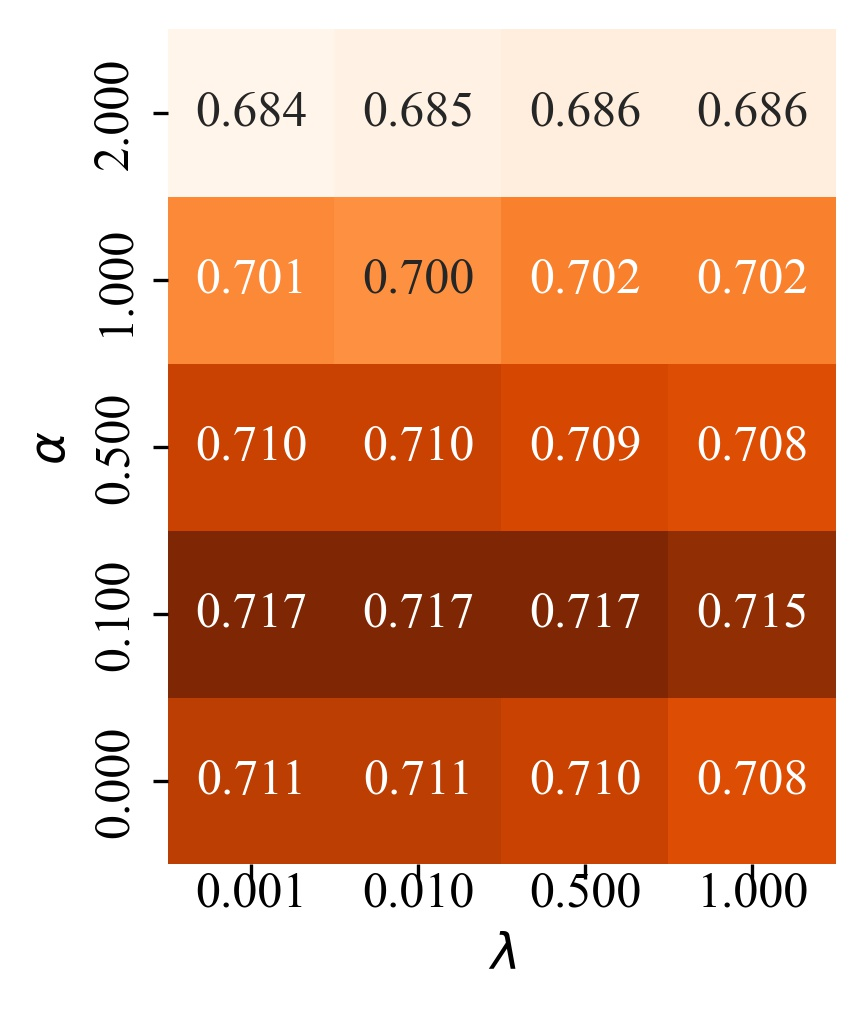}
        \caption{\sensitivity}
    \end{subfigure}%
    
    \begin{subfigure}{0.32\textwidth}
        \centering
        \includegraphics[width=\textwidth]{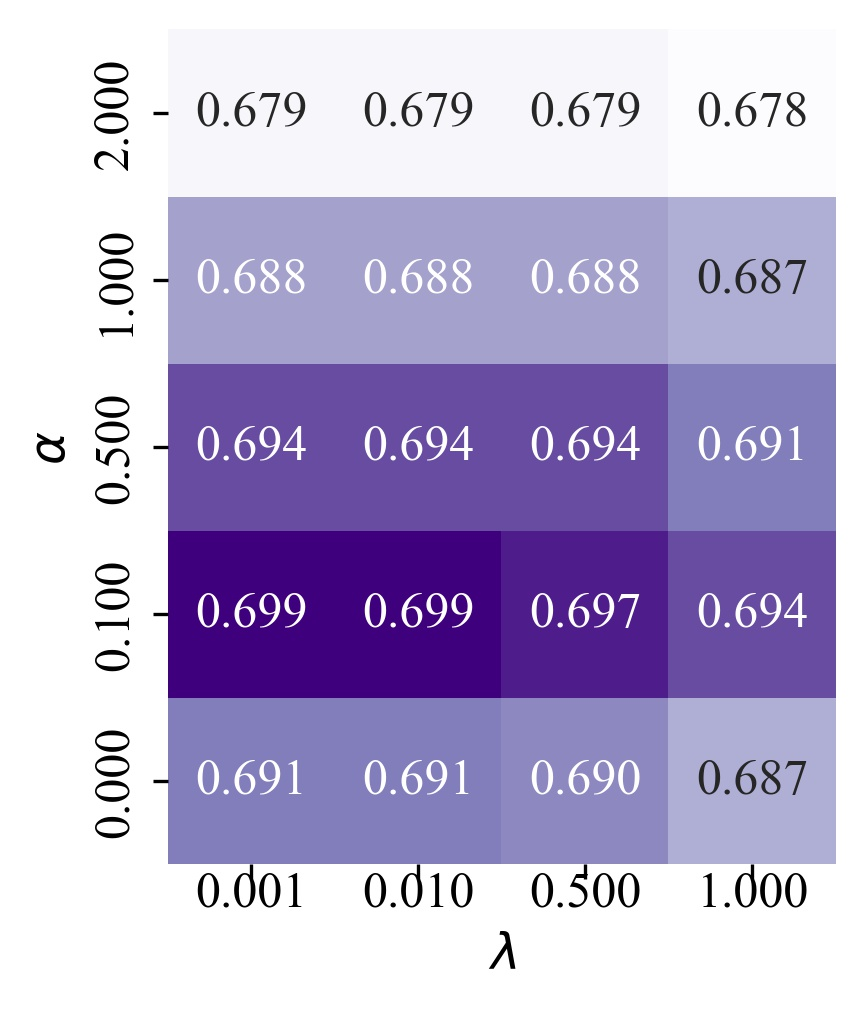}
        \caption{\accuracy}
    \end{subfigure}
     ~ 
    \begin{subfigure}{0.32\textwidth}
        \centering
        \includegraphics[width=\textwidth]{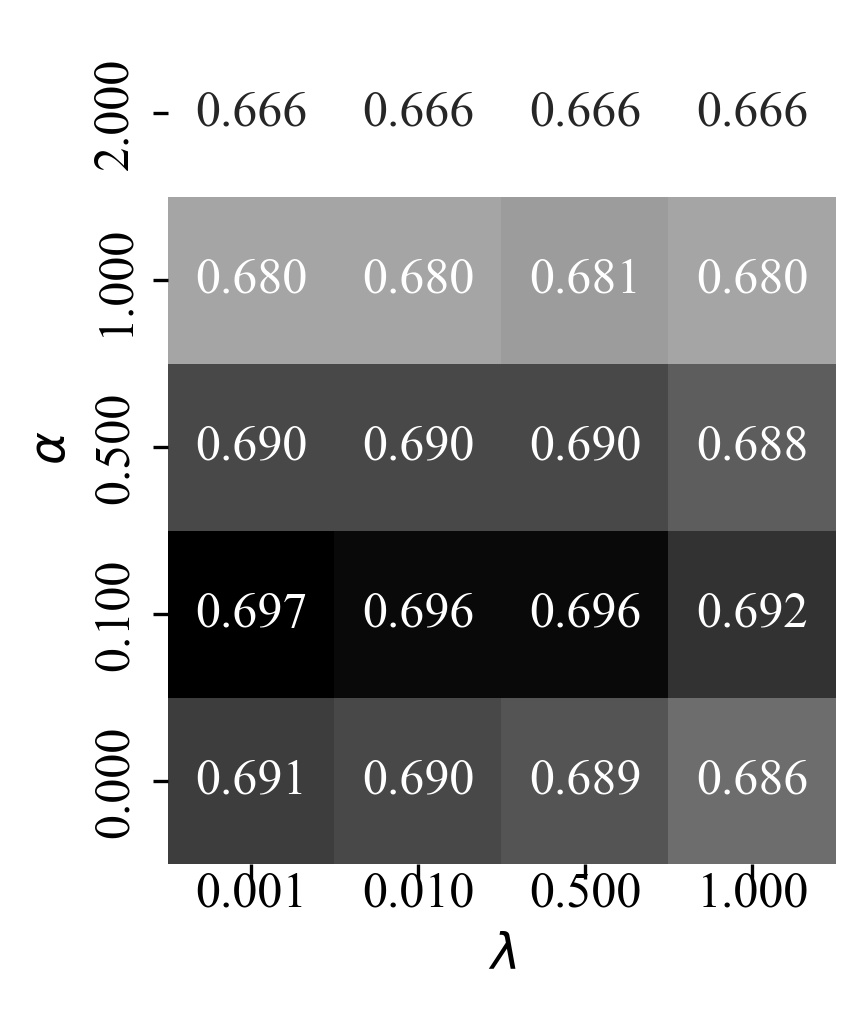}
        \caption{\fone score}
    \end{subfigure}
    \caption{Parameter Study of \OurMethodWithDMPNNAWithDisc}
    \label{supp:fig:param_best_tasks_aada_dmpnna_LG}
\end{figure*}
