# Supplementary material for: Improving Compound Activity Classification via Deep Transfer and Representation Learning
Source: arXiv:2111.07439 source file (2022-03-09)
Supplement: Supplementary file 2 [file supp.pdf]

# Improving Compound Activity Classification via Deep Transfer and Representation Learning (Supplementary Materials)

Vishal Dey,<sup>†</sup> Raghu Machiraju,<sup>†,‡,¶</sup> and Xia Ning<sup>\*,†,‡,¶</sup>

<sup>†</sup>*Department of Computer Science and Engineering, The Ohio State University, Columbus, OH*

<sup>‡</sup>*Biomedical Informatics, The Ohio State University, Columbus, OH*

<sup>¶</sup>*Translational Data Analytics Institute, The Ohio State University, Columbus, OH*

E-mail: ning.104@osu.edu

## 1 Directed Message Passing Neural Networks

**dmpn** incorporates atom features  $\mathbf{a}_u$  for each atom  $u \in \mathcal{A}_c$  and bond features  $\mathbf{e}_{uv}$  for each bond  $(u, v) \in \mathcal{E}_c$ , and captures molecular substructures by propagating messages along directed edges in  $\mathcal{G}_c$ . **dmpn** initializes atom features  $\mathbf{a}_u$  using the atom’s physicochemical properties including mass, formal charge, chirality, type, number of connected bonds, etc. **dmpn** initializes bond features  $\mathbf{e}_{uv}$  using bond type, stereo configuration, etc.

In particular, in  $\mathcal{G}_c$ , each bond  $(u, v)$  is associated with two messages  $\mathbf{m}_{uv}$  and  $\mathbf{m}_{vu}$  encoding messages from atom  $u$  to  $v$  and vice versa. Each message  $\mathbf{m}_{uv}^{(t+1)}$  in the  $(t + 1)$ -th

iteration of **dmpn** is aggregated as follows,

$$\mathbf{m}_{uv}^{(t+1)} = \sum_{k \in \mathcal{N}(u) \setminus v} \mathbf{h}_{ku}^{(t)} \quad (1)$$

where  $\mathcal{N}(u)$  is the set of atoms connected to  $u$ ,  $\mathbf{h}_{ku}^{(t)}$  is the hidden state of edge  $(k, u)$  in the  $t$ -th iteration. In the  $(t + 1)$ -th iteration of message passing, the hidden state  $\mathbf{h}_{uv}^{(t+1)}$  for each edge  $(u, v)$  is updated as follows,

$$\mathbf{h}_{uv}^{(t+1)} = \text{ReLU}(\mathbf{h}_{uv}^{(0)} + W\mathbf{m}_{uv}^{(t+1)}), \quad (2)$$

where  $W$  is a learnable parameter matrix, and  $\mathbf{h}_{uv}^{(0)}$  is the initial hidden state of edge  $(u, v)$  initialized as follows,

$$\mathbf{h}_{uv}^{(0)} = \text{ReLU}(W_0[\mathbf{a}_u, \mathbf{e}_{uv}]) \quad (3)$$

where  $\mathbf{a}_u$  and  $\mathbf{e}_{uv}$  are atom and bond feature vectors, respectively,  $[\mathbf{a}_u, \mathbf{e}_{uv}]$  is the concatenation of  $\mathbf{a}_u$  and  $\mathbf{e}_{uv}$  and  $W_0$  is a learnable parameter.

After the final iteration of message passing, the hidden states for edges incident to an atom  $u$  are aggregated to generate an intermediate representation  $\mathbf{h}_u$  for that atom as follows,

$$\mathbf{h}_u = \sum_{k \in \mathcal{N}(u)} \mathbf{h}_{ku}^{(\tau)}, \quad (4)$$

where  $\tau$  is the total number of message passing iterations. These intermediate atom representations are then used to generate another atom representation that also incorporates atom features  $\mathbf{a}_u$  as follows,

$$\mathbf{s}_u = \text{ReLU}(W_e[\mathbf{a}_u, \mathbf{h}_u]), \quad (5)$$

where  $W_e$  is a learnable parameter and  $[\mathbf{a}_u, \mathbf{h}_u]$  is the concatenation of  $\mathbf{a}_u$  and  $\mathbf{h}_u$ . Thus, the atom representation  $\mathbf{h}_u$  captures structural information about atom  $u$ 's  $\tau$ -hop neighbors, thereby enhancing the representation power. Given the representation  $\mathbf{h}_u$  for each atom in

$c$ , `dmpn` produces an embedding for  $c$  using mean pooling over all the atom representations as follows,

$$\mathbf{r}_c = \frac{1}{|\mathcal{A}_c|} \sum_{u \in \mathcal{A}_c} \mathbf{s}_u, \quad (6)$$

where  $|\mathcal{A}_c|$  is the number of atoms in  $c$ .

## 2 Supplementary Materials

### 2.1 Assay Information

Table S1 presents the assay statistics of 93 processed bioassays with their associated target protein accession IDs in PubChem; their number of total, active and inactive compounds, and the corresponding protein family for each associated target.

Table S1: Compound statistics of processed bioassays

| protacxn     | #total  | # active | # inactive | Protein family                      |
|--------------|---------|----------|------------|-------------------------------------|
| NP_001017535 | 380,711 | 5,152    | 375,559    | Nuclear hormone receptor family     |
| AAH18745     | 374,923 | 1,230    | 373,693    | Peptidase family                    |
| NP_005021    | 349,900 | 10,198   | 339,702    | Protein kinase superfamily          |
| NP_004196    | 336,578 | 238      | 336,340    | Peptidase family                    |
| NP_057051    | 292,415 | 97       | 292,318    | Protein-tyrosine phosphatase family |
| NP_000903    | 292,382 | 151      | 292,231    | G-protein coupled receptor 1 family |
| NP_005292    | 292,044 | 207      | 291,837    | G-protein coupled receptor 1 family |
| NP_004081    | 290,998 | 1,674    | 289,324    | Protein-tyrosine phosphatase family |
| NP_001121649 | 275,994 | 116      | 275,878    | Nuclear hormone receptor family     |
| NP_997055    | 208,843 | 2,526    | 206,317    | G-protein coupled receptor 1 family |
| NP_002736    | 182,123 | 1,207    | 180,916    | Protein kinase superfamily          |

Continued on next page

**Table S1 – continued from previous page**

| protacxn               | #total  | # active | # inactive | Protein family                      |
|------------------------|---------|----------|------------|-------------------------------------|
| NP_542155              | 112,687 | 906      | 111,781    | Protein-tyrosine phosphatase family |
| NP_775180              | 96,456  | 153      | 96,303     | Nuclear hormone receptor family     |
| P55210                 | 71,790  | 77       | 71,713     | Peptidase family                    |
| NP_150634              | 70,986  | 61       | 70,925     | Peptidase family                    |
| NP_000483              | 10,100  | 179      | 9,921      | ABC transporter superfamily         |
| ABB72139               | 6,968   | 64       | 6,904      | Nuclear hormone receptor family     |
| ADZ17337               | 6,738   | 86       | 6,652      | Nuclear hormone receptor family     |
| NP_000762              | 7,759   | 1,163    | 6,596      | Cytochrome P450 family              |
| EAW77416               | 7,131   | 626      | 6,505      | Cytochrome P450 family              |
| ADZ17384               | 6,425   | 55       | 6,370      | Nuclear hormone receptor family     |
| NP_000760              | 7,676   | 1,713    | 5,963      | Cytochrome P450 family              |
| NP_000752              | 7,670   | 4,008    | 3,662      | Cytochrome P450 family              |
| AAF64255               | 2,728   | 1,107    | 1,621      | Bcl-2 family                        |
| NP_002084              | 2,285   | 682      | 1,603      | Protein kinase superfamily          |
| NP_063937              | 2,390   | 823      | 1,567      | Protein kinase superfamily          |
| AAI28575               | 1,824   | 305      | 1,519      | Nuclear hormone receptor family     |
| AAB26273               | 1,669   | 276      | 1,393      | G-protein coupled receptor 1 family |
| NP_000947              | 1,350   | 139      | 1,211      | G-protein coupled receptor 1 family |
| NP_036559              | 1,260   | 109      | 1,151      | Peptidase family                    |
| NP_065717              | 1,630   | 661      | 969        | Protein kinase superfamily          |
| AAI27629               | 1,065   | 160      | 905        | G-protein coupled receptor 1 family |
| P51449                 | 978     | 138      | 840        | Nuclear hormone receptor family     |
| NP_004040              | 824     | 91       | 733        | Bcl-2 family                        |
| Continued on next page |         |          |            |                                     |

**Table S1 – continued from previous page**

| protacxn               | #total | # active | # inactive | Protein family                      |
|------------------------|--------|----------|------------|-------------------------------------|
| P00748                 | 761    | 160      | 601        | Peptidase family                    |
| ABD72211               | 1,164  | 605      | 559        | ABC transporter superfamily         |
| AAH04460               | 993    | 445      | 548        | Peptidase family                    |
| NP_004950              | 954    | 456      | 498        | Nuclear hormone receptor family     |
| NP_000676              | 667    | 209      | 458        | G-protein coupled receptor 1 family |
| NP_000466              | 489    | 55       | 434        | Nuclear hormone receptor family     |
| NP_005152              | 672    | 259      | 413        | G-protein coupled receptor 1 family |
| NP_001391              | 729    | 345      | 384        | G-protein coupled receptor 1 family |
| NP_005217              | 456    | 82       | 374        | G-protein coupled receptor 1 family |
| NP_660205              | 1,167  | 795      | 372        | Peptidase family                    |
| NP_000789              | 457    | 100      | 357        | G-protein coupled receptor 1 family |
| NP_001027450           | 543    | 203      | 340        | Peptidase family                    |
| NP_004521              | 445    | 107      | 338        | Peptidase family                    |
| NP_004960              | 387    | 61       | 326        | Peptidase family                    |
| NP_005424              | 693    | 368      | 325        | Protein kinase superfamily          |
| P53779                 | 362    | 57       | 305        | Protein kinase superfamily          |
| AAC63054               | 517    | 223      | 294        | Peptidase family                    |
| AAF04852               | 973    | 683      | 290        | Peptidase family                    |
| NP_004337              | 1,055  | 781      | 274        | Peptidase family                    |
| AAA51985               | 366    | 105      | 261        | Peptidase family                    |
| NP_004358              | 289    | 58       | 231        | G-protein coupled receptor 1 family |
| NP_004221              | 276    | 69       | 207        | G-protein coupled receptor 1 family |
| NP_000901              | 292    | 88       | 204        | G-protein coupled receptor 1 family |
| Continued on next page |        |          |            |                                     |

**Table S1 – continued from previous page**

| protacxn               | #total | # active | # inactive | Protein family                      |
|------------------------|--------|----------|------------|-------------------------------------|
| NP_002522              | 349    | 156      | 193        | G-protein coupled receptor 1 family |
| NP_644806              | 248    | 57       | 191        | Peptidase family                    |
| EAW86722               | 539    | 350      | 189        | G-protein coupled receptor 1 family |
| NP_000900              | 291    | 104      | 187        | G-protein coupled receptor 1 family |
| AAI07736               | 242    | 59       | 183        | Bcl-2 family                        |
| AAI29989               | 981    | 799      | 182        | Peptidase family                    |
| BAH02301               | 462    | 317      | 145        | Nuclear hormone receptor family     |
| NP_000448              | 292    | 149      | 143        | Nuclear hormone receptor family     |
| NP_004841              | 229    | 88       | 141        | Protein kinase superfamily          |
| AAH14970               | 248    | 126      | 122        | G-protein coupled receptor 1 family |
| NP_002721              | 190    | 71       | 119        | Protein kinase superfamily          |
| NP_003813              | 211    | 92       | 119        | Nuclear hormone receptor family     |
| AAH36651               | 210    | 92       | 118        | Protein kinase superfamily          |
| Q05397                 | 210    | 110      | 100        | Protein kinase superfamily          |
| NP_004570              | 151    | 52       | 99         | Protein kinase superfamily          |
| NP_000918              | 189    | 102      | 87         | ABC transporter superfamily         |
| NP_112168              | 304    | 217      | 87         | Protein kinase superfamily          |
| NP_066285              | 233    | 173      | 60         | Nuclear hormone receptor family     |
| BAB91222               | 142    | 91       | 51         | G-protein coupled receptor 1 family |
| NP_003605              | 232    | 181      | 51         | G-protein coupled receptor 1 family |
| P28566                 | 95     | 51       | 44         | G-protein coupled receptor 1 family |
| NP_037457              | 331    | 290      | 41         | Peptidase family                    |
| Q6L5J4                 | 432    | 391      | 41         | G-protein coupled receptor 1 family |
| Continued on next page |        |          |            |                                     |

**Table S1 – continued from previous page**

| protacxn     | #total | # active | # inactive | Protein family                      |
|--------------|--------|----------|------------|-------------------------------------|
| NP_000732    | 98     | 58       | 40         | G-protein coupled receptor 1 family |
| NP_612200    | 314    | 274      | 40         | G-protein coupled receptor 1 family |
| NP_001387    | 307    | 270      | 37         | Protein kinase superfamily          |
| NP_004818    | 125    | 89       | 36         | ABC transporter superfamily         |
| EAW70217     | 188    | 154      | 34         | Protein kinase superfamily          |
| AAH14460     | 91     | 69       | 22         | Peptidase family                    |
| NP_001124480 | 81     | 64       | 17         | Protein-tyrosine phosphatase family |
| NP_001516    | 171    | 156      | 15         | G-protein coupled receptor 1 family |
| NP_003984    | 95     | 83       | 12         | Protein kinase superfamily          |
| NP_004705    | 94     | 82       | 12         | Protein kinase superfamily          |
| NP_004062    | 96     | 88       | 8          | Protein kinase superfamily          |
| NP_002825    | 166    | 160      | 6          | Protein-tyrosine phosphatase family |
| NP_004942    | 74     | 69       | 5          | G-protein coupled receptor 1 family |

In this table, the columns protacxn, #total, #active and #inactive correspond to the target protein’s accession number from PubChem, number of total compounds, active compounds and inactive compounds in the bioassay, respectively. The column Protein family denotes the corresponding protein family for each target.

## 2.2 Assay Pairs Information

Table S2 presents the compound statistics of all 120 pairs in  $\mathcal{P}$  with their number of total, active and inactive compounds in each assay of every pair.

Table S2: Compound statistics of selected bioassay pairs

| target(P) | target(Q) | $ \mathcal{X}_{B_P} $ | $ \mathcal{X}_{B_P}^+ $ | $ \mathcal{X}_{B_P}^- $ | $ \mathcal{X}_{B_Q} $ | $ \mathcal{X}_{B_Q}^+ $ | $ \mathcal{X}_{B_Q}^- $ |
|-----------|-----------|-----------------------|-------------------------|-------------------------|-----------------------|-------------------------|-------------------------|
| NP_005021 | NP_004705 | 20,396                | 10,198                  | 10,198                  | 164                   | 82                      | 82                      |
| NP_000903 | EAW86722  | 302                   | 151                     | 151                     | 666                   | 333                     | 333                     |
| NP_000903 | BAB91222  | 302                   | 151                     | 151                     | 166                   | 83                      | 83                      |
| NP_005292 | BAB91222  | 414                   | 207                     | 207                     | 166                   | 83                      | 83                      |
| NP_005292 | NP_004942 | 414                   | 207                     | 207                     | 134                   | 67                      | 67                      |
| NP_004081 | NP_002825 | 3,288                 | 1,644                   | 1,644                   | 248                   | 124                     | 124                     |
| NP_997055 | NP_004942 | 5,052                 | 2,526                   | 2,526                   | 134                   | 67                      | 67                      |
| NP_775180 | ADZ17337  | 306                   | 153                     | 153                     | 170                   | 85                      | 85                      |
| NP_000483 | ABD72211  | 356                   | 178                     | 178                     | 1,188                 | 594                     | 594                     |
| NP_000483 | NP_000918 | 358                   | 179                     | 179                     | 204                   | 102                     | 102                     |
| NP_000483 | NP_004818 | 358                   | 179                     | 179                     | 178                   | 89                      | 89                      |
| ADZ17337  | AAI28575  | 156                   | 78                      | 78                      | 592                   | 296                     | 296                     |
| ADZ17337  | NP_000448 | 172                   | 86                      | 86                      | 298                   | 149                     | 149                     |
| ADZ17337  | NP_066285 | 172                   | 86                      | 86                      | 342                   | 171                     | 171                     |
| NP_000762 | NP_000752 | 888                   | 444                     | 444                     | 1,918                 | 959                     | 959                     |
| NP_000760 | NP_000752 | 1,356                 | 678                     | 678                     | 2,070                 | 1,035                   | 1,035                   |
| NP_002084 | P53779    | 1,358                 | 679                     | 679                     | 112                   | 56                      | 56                      |
| AAI28575  | P51449    | 608                   | 304                     | 304                     | 244                   | 122                     | 122                     |
| AAI28575  | BAH02301  | 608                   | 304                     | 304                     | 626                   | 313                     | 313                     |
| AAI28575  | NP_000448 | 608                   | 304                     | 304                     | 298                   | 149                     | 149                     |
| AAI28575  | NP_066285 | 610                   | 305                     | 305                     | 346                   | 173                     | 173                     |
| AAB26273  | NP_000947 | 536                   | 268                     | 268                     | 272                   | 136                     | 136                     |
| AAB26273  | AAI27629  | 552                   | 276                     | 276                     | 320                   | 160                     | 160                     |

Continued on next page



**Table S2 – continued from previous page**

| target(P) | target(Q) | $ \mathcal{X}_{B_P} $ | $ \mathcal{X}_{B_P}^+ $ | $ \mathcal{X}_{B_P}^- $ | $ \mathcal{X}_{B_Q} $ | $ \mathcal{X}_{B_Q}^+ $ | $ \mathcal{X}_{B_Q}^- $ |
|-----------|-----------|-----------------------|-------------------------|-------------------------|-----------------------|-------------------------|-------------------------|
| AAB26273  | NP_000676 | 552                   | 276                     | 276                     | 416                   | 208                     | 208                     |
| AAB26273  | NP_001391 | 548                   | 274                     | 274                     | 688                   | 344                     | 344                     |
| AAB26273  | NP_004358 | 552                   | 276                     | 276                     | 116                   | 58                      | 58                      |
| AAB26273  | NP_000901 | 552                   | 276                     | 276                     | 174                   | 87                      | 87                      |
| AAB26273  | EAW86722  | 552                   | 276                     | 276                     | 700                   | 350                     | 350                     |
| AAB26273  | NP_000900 | 552                   | 276                     | 276                     | 206                   | 103                     | 103                     |
| AAB26273  | AAH14970  | 552                   | 276                     | 276                     | 252                   | 126                     | 126                     |
| AAB26273  | BAB91222  | 552                   | 276                     | 276                     | 182                   | 91                      | 91                      |
| AAB26273  | NP_003605 | 552                   | 276                     | 276                     | 360                   | 180                     | 180                     |
| AAB26273  | NP_612200 | 552                   | 276                     | 276                     | 542                   | 271                     | 271                     |
| AAB26273  | NP_001516 | 552                   | 276                     | 276                     | 310                   | 155                     | 155                     |
| NP_000947 | AAI27629  | 278                   | 139                     | 139                     | 318                   | 159                     | 159                     |
| NP_000947 | EAW86722  | 278                   | 139                     | 139                     | 700                   | 350                     | 350                     |
| NP_000947 | BAB91222  | 278                   | 139                     | 139                     | 182                   | 91                      | 91                      |
| NP_000947 | NP_001516 | 278                   | 139                     | 139                     | 308                   | 154                     | 154                     |
| NP_036559 | P00748    | 168                   | 84                      | 84                      | 274                   | 137                     | 137                     |
| NP_036559 | AAC63054  | 184                   | 92                      | 92                      | 410                   | 205                     | 205                     |
| NP_036559 | AAF04852  | 218                   | 109                     | 109                     | 1,362                 | 681                     | 681                     |
| NP_036559 | NP_004337 | 218                   | 109                     | 109                     | 1,556                 | 778                     | 778                     |
| NP_036559 | AAA51985  | 174                   | 87                      | 87                      | 180                   | 90                      | 90                      |
| NP_036559 | AAI29989  | 218                   | 109                     | 109                     | 1,592                 | 796                     | 796                     |
| NP_036559 | AAH14460  | 202                   | 101                     | 101                     | 120                   | 60                      | 60                      |
| NP_065717 | NP_001387 | 1,028                 | 514                     | 514                     | 278                   | 139                     | 139                     |

Continued on next page

**Table S2 – continued from previous page**

| target(P) | target(Q) | $ \mathcal{X}_{B_P} $ | $ \mathcal{X}_{B_P}^+ $ | $ \mathcal{X}_{B_P}^- $ | $ \mathcal{X}_{B_Q} $ | $ \mathcal{X}_{B_Q}^+ $ | $ \mathcal{X}_{B_Q}^- $ |
|-----------|-----------|-----------------------|-------------------------|-------------------------|-----------------------|-------------------------|-------------------------|
| NP_065717 | EAW70217  | 1,268                 | 634                     | 634                     | 260                   | 130                     | 130                     |
| AAI27629  | EAW86722  | 320                   | 160                     | 160                     | 698                   | 349                     | 349                     |
| AAI27629  | NP_004942 | 320                   | 160                     | 160                     | 138                   | 69                      | 69                      |
| P00748    | NP_660205 | 320                   | 160                     | 160                     | 1,586                 | 793                     | 793                     |
| P00748    | NP_004521 | 320                   | 160                     | 160                     | 214                   | 107                     | 107                     |
| P00748    | AAC63054  | 266                   | 133                     | 133                     | 382                   | 191                     | 191                     |
| P00748    | AAF04852  | 320                   | 160                     | 160                     | 1,364                 | 682                     | 682                     |
| P00748    | NP_004337 | 320                   | 160                     | 160                     | 1,558                 | 779                     | 779                     |
| P00748    | AAA51985  | 244                   | 122                     | 122                     | 154                   | 77                      | 77                      |
| P00748    | AAI29989  | 320                   | 160                     | 160                     | 1,596                 | 798                     | 798                     |
| P00748    | AAH14460  | 296                   | 148                     | 148                     | 114                   | 57                      | 57                      |
| ABD72211  | NP_000918 | 1,210                 | 605                     | 605                     | 202                   | 101                     | 101                     |
| ABD72211  | NP_004818 | 1,210                 | 605                     | 605                     | 178                   | 89                      | 89                      |
| AAH04460  | AAH14460  | 890                   | 445                     | 445                     | 138                   | 69                      | 69                      |
| NP_000676 | NP_005152 | 154                   | 77                      | 77                      | 172                   | 86                      | 86                      |
| NP_000676 | NP_000901 | 416                   | 208                     | 208                     | 176                   | 88                      | 88                      |
| NP_000676 | EAW86722  | 418                   | 209                     | 209                     | 700                   | 350                     | 350                     |
| NP_000676 | NP_001516 | 418                   | 209                     | 209                     | 310                   | 155                     | 155                     |
| NP_000676 | NP_004942 | 418                   | 209                     | 209                     | 138                   | 69                      | 69                      |
| NP_005152 | NP_004358 | 512                   | 256                     | 256                     | 108                   | 54                      | 54                      |
| NP_005152 | NP_001516 | 518                   | 259                     | 259                     | 310                   | 155                     | 155                     |
| NP_001391 | NP_000901 | 682                   | 341                     | 341                     | 174                   | 87                      | 87                      |
| NP_001391 | EAW86722  | 690                   | 345                     | 345                     | 700                   | 350                     | 350                     |

Continued on next page

**Table S2 – continued from previous page**

| target(P) | target(Q) | $ \mathcal{X}_{B_P} $ | $ \mathcal{X}_{B_P}^+ $ | $ \mathcal{X}_{B_P}^- $ | $ \mathcal{X}_{B_Q} $ | $ \mathcal{X}_{B_Q}^+ $ | $ \mathcal{X}_{B_Q}^- $ |
|-----------|-----------|-----------------------|-------------------------|-------------------------|-----------------------|-------------------------|-------------------------|
| NP_001391 | NP_000900 | 682                   | 341                     | 341                     | 206                   | 103                     | 103                     |
| NP_001391 | BAB91222  | 690                   | 345                     | 345                     | 182                   | 91                      | 91                      |
| NP_001391 | NP_001516 | 690                   | 345                     | 345                     | 308                   | 154                     | 154                     |
| NP_660205 | NP_004337 | 914                   | 457                     | 457                     | 642                   | 321                     | 321                     |
| NP_660205 | AAI29989  | 986                   | 493                     | 493                     | 642                   | 321                     | 321                     |
| NP_005424 | NP_001387 | 736                   | 368                     | 368                     | 540                   | 270                     | 270                     |
| NP_005424 | NP_003984 | 736                   | 368                     | 368                     | 166                   | 83                      | 83                      |
| NP_005424 | NP_004705 | 736                   | 368                     | 368                     | 164                   | 82                      | 82                      |
| NP_005424 | NP_004062 | 736                   | 368                     | 368                     | 176                   | 88                      | 88                      |
| AAC63054  | AAF04852  | 446                   | 223                     | 223                     | 1,364                 | 682                     | 682                     |
| AAC63054  | NP_004337 | 446                   | 223                     | 223                     | 1,558                 | 779                     | 779                     |
| AAC63054  | AAA51985  | 402                   | 201                     | 201                     | 182                   | 91                      | 91                      |
| AAC63054  | AAI29989  | 446                   | 223                     | 223                     | 1,594                 | 797                     | 797                     |
| AAC63054  | AAH14460  | 438                   | 219                     | 219                     | 130                   | 65                      | 65                      |
| AAF04852  | NP_004337 | 654                   | 327                     | 327                     | 718                   | 359                     | 359                     |
| AAF04852  | AAI29989  | 682                   | 341                     | 341                     | 696                   | 348                     | 348                     |
| NP_004337 | AAI29989  | 804                   | 402                     | 402                     | 758                   | 379                     | 379                     |
| AAA51985  | AAI29989  | 210                   | 105                     | 105                     | 1,598                 | 799                     | 799                     |
| AAA51985  | AAH14460  | 194                   | 97                      | 97                      | 118                   | 59                      | 59                      |
| NP_004358 | NP_000901 | 116                   | 58                      | 58                      | 176                   | 88                      | 88                      |
| NP_004358 | EAW86722  | 116                   | 58                      | 58                      | 700                   | 350                     | 350                     |
| NP_004358 | NP_000900 | 116                   | 58                      | 58                      | 208                   | 104                     | 104                     |
| NP_004358 | AAH14970  | 116                   | 58                      | 58                      | 244                   | 122                     | 122                     |

Continued on next page

**Table S2 – continued from previous page**

| target(P) | target(Q) | $ \mathcal{X}_{B_P} $ | $ \mathcal{X}_{B_P}^+ $ | $ \mathcal{X}_{B_P}^- $ | $ \mathcal{X}_{B_Q} $ | $ \mathcal{X}_{B_Q}^+ $ | $ \mathcal{X}_{B_Q}^- $ |
|-----------|-----------|-----------------------|-------------------------|-------------------------|-----------------------|-------------------------|-------------------------|
| NP_004358 | BAB91222  | 116                   | 58                      | 58                      | 182                   | 91                      | 91                      |
| NP_004358 | NP_001516 | 116                   | 58                      | 58                      | 312                   | 156                     | 156                     |
| NP_004221 | EAW86722  | 138                   | 69                      | 69                      | 700                   | 350                     | 350                     |
| NP_004221 | NP_001516 | 138                   | 69                      | 69                      | 312                   | 156                     | 156                     |
| NP_004221 | NP_004942 | 138                   | 69                      | 69                      | 138                   | 69                      | 69                      |
| NP_000901 | EAW86722  | 174                   | 87                      | 87                      | 700                   | 350                     | 350                     |
| NP_000901 | BAB91222  | 176                   | 88                      | 88                      | 182                   | 91                      | 91                      |
| NP_000901 | NP_001516 | 176                   | 88                      | 88                      | 312                   | 156                     | 156                     |
| EAW86722  | AAH14970  | 700                   | 350                     | 350                     | 250                   | 125                     | 125                     |
| EAW86722  | BAB91222  | 700                   | 350                     | 350                     | 182                   | 91                      | 91                      |
| EAW86722  | NP_001516 | 700                   | 350                     | 350                     | 312                   | 156                     | 156                     |
| NP_000900 | BAB91222  | 208                   | 104                     | 104                     | 182                   | 91                      | 91                      |
| NP_000900 | NP_001516 | 208                   | 104                     | 104                     | 312                   | 156                     | 156                     |
| NP_000900 | NP_004942 | 208                   | 104                     | 104                     | 138                   | 69                      | 69                      |
| AAH14970  | BAB91222  | 252                   | 126                     | 126                     | 182                   | 91                      | 91                      |
| AAH14970  | NP_001516 | 252                   | 126                     | 126                     | 310                   | 155                     | 155                     |
| AAH14970  | NP_004942 | 252                   | 126                     | 126                     | 138                   | 69                      | 69                      |
| NP_002721 | NP_001387 | 142                   | 71                      | 71                      | 540                   | 270                     | 270                     |
| NP_002721 | NP_003984 | 142                   | 71                      | 71                      | 166                   | 83                      | 83                      |
| NP_002721 | NP_004705 | 142                   | 71                      | 71                      | 164                   | 82                      | 82                      |
| NP_002721 | NP_004062 | 142                   | 71                      | 71                      | 176                   | 88                      | 88                      |
| BAB91222  | NP_004942 | 182                   | 91                      | 91                      | 138                   | 69                      | 69                      |
| NP_003605 | NP_004942 | 362                   | 181                     | 181                     | 138                   | 69                      | 69                      |

Continued on next page

**Table S2 – continued from previous page**

| target(P)    | target(Q) | $ \mathcal{X}_{B_P} $ | $ \mathcal{X}_{B_P}^+ $ | $ \mathcal{X}_{B_P}^- $ | $ \mathcal{X}_{B_Q} $ | $ \mathcal{X}_{B_Q}^+ $ | $ \mathcal{X}_{B_Q}^- $ |
|--------------|-----------|-----------------------|-------------------------|-------------------------|-----------------------|-------------------------|-------------------------|
| NP_001387    | EAW70217  | 488                   | 244                     | 244                     | 260                   | 130                     | 130                     |
| EAW70217     | NP_003984 | 278                   | 139                     | 139                     | 136                   | 68                      | 68                      |
| EAW70217     | NP_004705 | 280                   | 140                     | 140                     | 132                   | 66                      | 66                      |
| EAW70217     | NP_004062 | 280                   | 140                     | 140                     | 142                   | 71                      | 71                      |
| NP_001124480 | NP_002825 | 128                   | 64                      | 64                      | 318                   | 159                     | 159                     |

In this table, the first two columns target(P) and target(Q) correspond to the accession numbers of the two target proteins corresponding to the two bioassays P and Q of the pair, respectively. The columns  $|\mathcal{X}_{B_A}|$ ,  $|\mathcal{X}_{B_A}^+|$  and  $|\mathcal{X}_{B_A}^-|$  correspond to the number of total compounds, active compounds and inactive compounds in the bioassay  $A$  where ( $A = \{P, Q\}$  of each pair).

### 3 Supplementary Results

#### 3.1 Hyperparameter Configurations

Table S3: Hyperparameter Configurations

| parameter                         | values              |
|-----------------------------------|---------------------|
| $\alpha$                          | 0, 0.1, 0.5, 1, 2   |
| $\lambda$                         | 0.001, 0.01, 0.5, 1 |
| dimension $d$                     | 25, 50, 100         |
| # message passing steps $\tau$    | 2, 3, 4             |
| hidden layer size in $f_a(\cdot)$ | 100                 |
| hidden layer size in L, G and S   | 100                 |
| batch size                        | 10                  |
| learning rate                     | 1e-3                |

Table S3 presents the hyperparameter configurations for all our methods.  $\alpha$  and  $\lambda$  correspond to the trade-off parameter between the source and target classification losses as in

Equation 4) and the trade-off parameter between the classification and discriminator losses in Equation 13), respectively.  $\alpha$  is only associated with **TAc** and **TAc-fc**; whereas  $\lambda$  is only associated with **TAc-fc** and its variants. We tried 3 different values for  $d$  which represents the dimension of the compound representation out of **GNN** and **dmpna**; and 3 different values for the number of message passing steps  $\tau$ . Hence, these two hyperparameters are associated with all methods except **FCN-morgan** and **FCN-morganc**. The hidden layer size in the attention network denoted by  $f_a(\cdot)$ , the feature-wise discriminator denoted by **L**, and the compound-wise discriminator denoted by **G** is fixed to 100. We used a fixed batch size of 10 and an initial learning rate of 1e-3 with exponential decay every epoch from 1e-3 to 1e-4 at the end of training. We trained each model for 40 epochs with an early-stopping criteria based on the **ROC-AUC** performance on the validation set. Specifically, during training, we evaluated the **ROC-AUC** performance of each model on the validation set at every epoch; and we choose the trained model at some epoch  $k$  that gives the best performance on the validation set.

### 3.2 Prediction Analysis

Table S4 presents the pairwise similarity analysis for active compounds which were correctly classified by **TAc-c**, but incorrectly classified as inactive by **TAc**, **TAc-fc** and its variants.

Table S4: Similarity analysis of correct predictions by **TAc-c**

| source(S) | target(T) | #cor | #act | cor%   | $\text{sim}(\tilde{\mathcal{X}}_{B_T}^+, \mathcal{X}_{B_S}^+)$ | $\text{sim}(\tilde{\mathcal{X}}_{B_T}^+, \mathcal{X}_{B_T}^+)$ | sdiff%  | e-sdiff% | p-value  |
|-----------|-----------|------|------|--------|----------------------------------------------------------------|----------------------------------------------------------------|---------|----------|----------|
| EAW86722  | AAI27629  | 36   | 128  | 28.125 | 0.231                                                          | 0.194                                                          | 19.401  | 21.692   | 1.68e-05 |
| NP_004818 | ABD72211  | 131  | 485  | 27.010 | 0.191                                                          | 0.218                                                          | -12.557 | -12.312  | 3.05e-20 |
| NP_000901 | NP_001516 | 33   | 124  | 26.613 | 0.213                                                          | 0.182                                                          | 17.135  | 19.886   | 2.57e-05 |
| NP_000483 | NP_000918 | 18   | 82   | 21.951 | 0.262                                                          | 0.444                                                          | -41.090 | -32.693  | 1.56e-05 |
| NP_004942 | NP_003605 | 29   | 145  | 20.000 | 0.164                                                          | 0.174                                                          | -5.916  | -2.832   | 4.15e-01 |
| NP_004221 | NP_001516 | 21   | 124  | 16.935 | 0.212                                                          | 0.203                                                          | 4.530   | 6.081    | 2.45e-01 |
| AAC63054  | AAF04852  | 85   | 546  | 15.568 | 0.255                                                          | 0.249                                                          | 2.490   | 3.969    | 1.25e-01 |

Continued on next page

Table S4 – continued from previous page

| source(S) | target(T) | #cor | #act | cor%   | $\text{sim}(\tilde{\mathcal{X}}_{B_T}^+, \mathcal{X}_{B_S}^+)$ | $\text{sim}(\tilde{\mathcal{X}}_{B_T}^+, \mathcal{X}_{B_T}^+)$ | sdiff%  | e-sdiff% | p-value  |
|-----------|-----------|------|------|--------|----------------------------------------------------------------|----------------------------------------------------------------|---------|----------|----------|
| NP_001516 | NP_000947 | 15   | 112  | 13.393 | 0.244                                                          | 0.193                                                          | 26.449  | 28.965   | 2.92e-04 |
| EAW86722  | NP_004358 | 6    | 46   | 13.043 | 0.239                                                          | 0.144                                                          | 66.156  | 66.256   | 5.06e-06 |
| AAH04460  | AAH14460  | 6    | 55   | 10.909 | 0.228                                                          | 0.154                                                          | 47.925  | 50.102   | 2.68e-05 |
| P00748    | NP_004521 | 8    | 85   | 9.412  | 0.227                                                          | 0.209                                                          | 8.621   | 11.614   | 2.38e-01 |
| P00748    | AAF04852  | 50   | 546  | 9.158  | 0.237                                                          | 0.267                                                          | -11.053 | -8.667   | 1.22e-04 |
| P00748    | NP_660205 | 57   | 634  | 8.991  | 0.243                                                          | 0.242                                                          | 0.662   | 1.593    | 6.55e-01 |
| NP_004942 | NP_000676 | 15   | 168  | 8.929  | 0.183                                                          | 0.216                                                          | -15.296 | -11.831  | 8.28e-03 |
| EAW86722  | NP_000947 | 10   | 112  | 8.929  | 0.240                                                          | 0.208                                                          | 15.663  | 17.138   | 1.41e-01 |
| AAC63054  | AAI29989  | 55   | 638  | 8.621  | 0.234                                                          | 0.249                                                          | -6.064  | -3.701   | 1.69e-02 |
| NP_001391 | NP_001516 | 10   | 123  | 8.130  | 0.269                                                          | 0.201                                                          | 33.649  | 34.022   | 1.13e-06 |
| EAW86722  | AAH14970  | 8    | 99   | 8.081  | 0.266                                                          | 0.212                                                          | 25.838  | 28.634   | 1.58e-02 |
| AAI29989  | AAF04852  | 22   | 273  | 8.059  | 0.315                                                          | 0.213                                                          | 48.214  | 50.797   | 3.80e-10 |
| NP_036559 | AAI29989  | 51   | 636  | 8.019  | 0.244                                                          | 0.258                                                          | -5.124  | -4.478   | 5.37e-03 |
| BAB91222  | AAH14970  | 8    | 101  | 7.921  | 0.175                                                          | 0.165                                                          | 5.943   | 8.653    | 3.60e-01 |
| P00748    | NP_036559 | 5    | 67   | 7.463  | 0.271                                                          | 0.184                                                          | 47.440  | 43.716   | 8.58e-02 |
| NP_004358 | AAH14970  | 7    | 98   | 7.143  | 0.207                                                          | 0.167                                                          | 24.161  | 23.704   | 9.37e-03 |
| AAA51985  | NP_036559 | 5    | 70   | 7.143  | 0.226                                                          | 0.167                                                          | 35.308  | 35.516   | 1.30e-03 |
| BAB91222  | NP_000901 | 5    | 71   | 7.042  | 0.252                                                          | 0.166                                                          | 51.322  | 52.216   | 2.77e-02 |
| NP_004358 | NP_001516 | 8    | 124  | 6.452  | 0.195                                                          | 0.196                                                          | -0.357  | 2.666    | 9.42e-01 |
| AAH14460  | AAC63054  | 11   | 176  | 6.250  | 0.240                                                          | 0.237                                                          | 1.395   | 4.762    | 8.31e-01 |
| NP_003984 | EAW70217  | 7    | 112  | 6.250  | 0.176                                                          | 0.207                                                          | -15.381 | -10.736  | 2.51e-01 |
| NP_001516 | NP_000676 | 10   | 168  | 5.952  | 0.215                                                          | 0.177                                                          | 21.813  | 25.027   | 4.71e-02 |
| NP_000900 | NP_001391 | 16   | 273  | 5.861  | 0.207                                                          | 0.187                                                          | 10.512  | 13.962   | 5.45e-02 |
| EAW86722  | NP_000901 | 4    | 70   | 5.714  | 0.211                                                          | 0.153                                                          | 37.288  | 39.267   | 3.66e-04 |
| NP_004062 | NP_005424 | 16   | 294  | 5.442  | 0.178                                                          | 0.191                                                          | -6.695  | -4.963   | 1.83e-01 |

Continued on next page

Table S4 – continued from previous page

| source(S) | target(T) | #cor | #act | cor%  | $\text{sim}(\tilde{\mathcal{X}}_{B_T}^+, \mathcal{X}_{B_S}^+)$ | $\text{sim}(\tilde{\mathcal{X}}_{B_T}^+, \mathcal{X}_{B_T}^+)$ | sdiff%  | e-sdiff% | p-value  |
|-----------|-----------|------|------|-------|----------------------------------------------------------------|----------------------------------------------------------------|---------|----------|----------|
| NP_001516 | AAB26273  | 12   | 222  | 5.405 | 0.192                                                          | 0.173                                                          | 11.478  | 13.326   | 2.22e-02 |
| AAH14460  | P00748    | 6    | 118  | 5.085 | 0.209                                                          | 0.176                                                          | 19.259  | 19.193   | 9.09e-03 |
| ADZ17337  | NP_000448 | 6    | 119  | 5.042 | 0.216                                                          | 0.378                                                          | -42.872 | -26.487  | 7.48e-02 |
| EAW86722  | AAB26273  | 11   | 222  | 4.955 | 0.171                                                          | 0.172                                                          | -0.639  | -0.201   | 9.25e-01 |
| AAB26273  | AAH14970  | 5    | 101  | 4.950 | 0.237                                                          | 0.191                                                          | 23.628  | 30.287   | 1.59e-01 |
| AAI28575  | ADZ17337  | 3    | 62   | 4.839 | 0.195                                                          | 0.122                                                          | 59.508  | 59.696   | 6.99e-03 |
| NP_004358 | AAB26273  | 10   | 222  | 4.505 | 0.180                                                          | 0.181                                                          | -0.222  | 1.167    | 9.65e-01 |
| P00748    | NP_004337 | 27   | 623  | 4.334 | 0.244                                                          | 0.271                                                          | -9.934  | -7.917   | 2.86e-03 |
| AAB26273  | NP_000901 | 3    | 70   | 4.286 | 0.200                                                          | 0.158                                                          | 26.692  | 33.966   | 1.20e-01 |
| AAB26273  | NP_000676 | 7    | 167  | 4.192 | 0.217                                                          | 0.294                                                          | -26.226 | -17.244  | 1.02e-01 |
| AAA51985  | P00748    | 4    | 98   | 4.082 | 0.254                                                          | 0.185                                                          | 37.324  | 38.576   | 3.26e-02 |
| AAA51985  | AAI29989  | 26   | 639  | 4.069 | 0.227                                                          | 0.243                                                          | -6.579  | -5.651   | 1.71e-02 |
| AAB26273  | EAW86722  | 11   | 280  | 3.929 | 0.253                                                          | 0.359                                                          | -29.579 | -7.283   | 1.26e-01 |
| NP_036559 | AAF04852  | 21   | 545  | 3.853 | 0.224                                                          | 0.237                                                          | -5.495  | -3.310   | 2.10e-01 |
| AAH14460  | AAH04460  | 13   | 356  | 3.652 | 0.154                                                          | 0.136                                                          | 12.702  | 12.870   | 1.06e-04 |
| NP_004358 | NP_000900 | 3    | 83   | 3.614 | 0.211                                                          | 0.181                                                          | 16.860  | 15.934   | 1.37e-01 |
| NP_000901 | EAW86722  | 10   | 280  | 3.571 | 0.251                                                          | 0.503                                                          | -50.099 | -46.770  | 1.25e-04 |
| NP_004818 | NP_000483 | 5    | 143  | 3.497 | 0.205                                                          | 0.190                                                          | 8.065   | 8.009    | 1.57e-01 |
| AAF04852  | AAC63054  | 6    | 179  | 3.352 | 0.318                                                          | 0.215                                                          | 48.069  | 49.310   | 5.66e-04 |
| AAI29989  | NP_660205 | 12   | 395  | 3.038 | 0.287                                                          | 0.191                                                          | 49.869  | 52.166   | 3.98e-05 |
| NP_775180 | ADZ17337  | 2    | 67   | 2.985 | 0.181                                                          | 0.143                                                          | 26.606  | 25.601   | 2.58e-01 |
| NP_000448 | ADZ17337  | 2    | 68   | 2.941 | 0.114                                                          | 0.060                                                          | 91.779  | 95.379   | 7.93e-02 |
| ADZ17337  | NP_066285 | 4    | 137  | 2.920 | 0.221                                                          | 0.204                                                          | 8.640   | 10.717   | 2.39e-01 |
| AAC63054  | NP_004337 | 18   | 623  | 2.889 | 0.264                                                          | 0.271                                                          | -2.731  | 0.234    | 5.85e-01 |
| NP_004358 | NP_000901 | 2    | 71   | 2.817 | 0.154                                                          | 0.123                                                          | 25.345  | 26.218   | 3.06e-01 |

Continued on next page



Table S4 – continued from previous page

| source(S) | target(T) | #cor | #act | cor%  | $\text{sim}(\tilde{\mathcal{X}}_{B_T}^+, \mathcal{X}_{B_S}^+)$ | $\text{sim}(\tilde{\mathcal{X}}_{B_T}^+, \mathcal{X}_{B_T}^+)$ | sdiff%  | e-sdiff% | p-value  |
|-----------|-----------|------|------|-------|----------------------------------------------------------------|----------------------------------------------------------------|---------|----------|----------|
| AAF04852  | NP_004337 | 8    | 287  | 2.787 | 0.321                                                          | 0.218                                                          | 47.407  | 50.401   | 6.15e-03 |
| AAB26273  | NP_000947 | 3    | 108  | 2.778 | 0.232                                                          | 0.158                                                          | 46.717  | 52.124   | 7.21e-02 |
| AAB26273  | NP_003605 | 4    | 144  | 2.778 | 0.219                                                          | 0.151                                                          | 44.746  | 43.328   | 3.17e-02 |
| NP_000901 | BAB91222  | 2    | 73   | 2.740 | 0.266                                                          | 0.584                                                          | -54.493 | -54.476  | 2.78e-02 |
| AAH14970  | AAB26273  | 6    | 222  | 2.703 | 0.191                                                          | 0.164                                                          | 16.190  | 16.216   | 7.96e-02 |
| BAB91222  | AAB26273  | 6    | 222  | 2.703 | 0.160                                                          | 0.167                                                          | -4.540  | -3.455   | 2.74e-01 |
| BAB91222  | NP_000947 | 3    | 112  | 2.679 | 0.206                                                          | 0.214                                                          | -3.745  | -2.894   | 7.53e-01 |
| P00748    | AAC63054  | 4    | 153  | 2.614 | 0.259                                                          | 0.249                                                          | 3.974   | 5.017    | 7.69e-01 |
| BAB91222  | NP_001391 | 7    | 276  | 2.536 | 0.158                                                          | 0.183                                                          | -13.803 | -13.149  | 1.29e-02 |
| AAH14460  | NP_036559 | 2    | 81   | 2.469 | 0.246                                                          | 0.186                                                          | 32.453  | 32.468   | 6.44e-02 |
| NP_004337 | P00748    | 3    | 128  | 2.344 | 0.270                                                          | 0.191                                                          | 41.575  | 43.957   | 1.01e-02 |
| AAI29989  | NP_036559 | 2    | 87   | 2.299 | 0.227                                                          | 0.150                                                          | 52.107  | 51.804   | 3.36e-01 |
| NP_004337 | AAC63054  | 4    | 179  | 2.235 | 0.283                                                          | 0.197                                                          | 43.357  | 42.784   | 4.74e-03 |
| NP_000760 | NP_000752 | 17   | 828  | 2.053 | 0.265                                                          | 0.197                                                          | 34.518  | 40.100   | 4.00e-05 |
| AAA51985  | AAC63054  | 3    | 160  | 1.875 | 0.263                                                          | 0.212                                                          | 24.034  | 24.481   | 8.67e-03 |
| NP_000903 | EAW86722  | 5    | 267  | 1.873 | 0.236                                                          | 0.507                                                          | -53.336 | -52.539  | 1.96e-03 |
| NP_000900 | AAB26273  | 4    | 222  | 1.802 | 0.192                                                          | 0.172                                                          | 11.874  | 21.471   | 5.88e-01 |
| NP_612200 | AAB26273  | 4    | 222  | 1.802 | 0.205                                                          | 0.192                                                          | 7.035   | 12.079   | 6.27e-01 |
| NP_004705 | EAW70217  | 2    | 112  | 1.786 | 0.176                                                          | 0.153                                                          | 15.465  | 15.582   | 3.20e-03 |
| AAI29989  | AAC63054  | 3    | 179  | 1.676 | 0.275                                                          | 0.195                                                          | 40.963  | 43.788   | 1.15e-01 |
| EAW86722  | NP_000903 | 2    | 121  | 1.653 | 0.201                                                          | 0.119                                                          | 68.483  | 73.823   | 1.13e-02 |
| BAH02301  | AAI28575  | 4    | 243  | 1.646 | 0.199                                                          | 0.155                                                          | 28.479  | 30.254   | 2.86e-02 |
| AAI29989  | P00748    | 2    | 128  | 1.563 | 0.307                                                          | 0.187                                                          | 63.821  | 68.477   | 2.76e-01 |
| NP_660205 | P00748    | 2    | 128  | 1.563 | 0.223                                                          | 0.199                                                          | 12.042  | 18.287   | 3.47e-01 |
| NP_000762 | NP_000752 | 11   | 768  | 1.432 | 0.252                                                          | 0.223                                                          | 12.713  | 16.400   | 7.20e-02 |

Continued on next page

Table S4 – continued from previous page

| source(S) | target(T) | #cor | #act  | cor%  | $\text{sim}(\tilde{\mathcal{X}}_{B_T}^+, \mathcal{X}_{B_S}^+)$ | $\text{sim}(\tilde{\mathcal{X}}_{B_T}^+, \mathcal{X}_{B_T}^+)$ | sdiff%  | e-sdiff% | p-value  |
|-----------|-----------|------|-------|-------|----------------------------------------------------------------|----------------------------------------------------------------|---------|----------|----------|
| BAB91222  | EAW86722  | 4    | 280   | 1.429 | 0.212                                                          | 0.395                                                          | -46.403 | -45.265  | 1.19e-02 |
| NP_000918 | NP_000483 | 2    | 143   | 1.399 | 0.181                                                          | 0.167                                                          | 8.313   | 8.153    | 2.06e-01 |
| NP_066285 | AAI28575  | 3    | 244   | 1.230 | 0.224                                                          | 0.175                                                          | 28.138  | 28.295   | 3.79e-02 |
| P00748    | AAI29989  | 7    | 638   | 1.097 | 0.234                                                          | 0.325                                                          | -27.930 | -17.446  | 1.11e-01 |
| AAB26273  | NP_001391 | 3    | 274   | 1.095 | 0.236                                                          | 0.220                                                          | 7.039   | 8.095    | 7.11e-01 |
| NP_004942 | NP_997055 | 19   | 2,020 | 0.941 | 0.174                                                          | 0.233                                                          | -25.354 | -24.636  | 1.43e-07 |
| NP_002721 | NP_001387 | 2    | 216   | 0.926 | 0.157                                                          | 0.262                                                          | -40.099 | -15.747  | 5.69e-01 |
| NP_001387 | NP_065717 | 3    | 411   | 0.730 | 0.303                                                          | 0.358                                                          | -15.284 | -11.201  | 3.77e-01 |
| AAF04852  | AAI29989  | 2    | 278   | 0.719 | 0.233                                                          | 0.190                                                          | 22.866  | 23.111   | 5.88e-02 |
| NP_000947 | EAW86722  | 2    | 280   | 0.714 | 0.219                                                          | 0.166                                                          | 31.671  | 31.738   | 6.30e-04 |
| NP_004337 | AAI29989  | 2    | 303   | 0.660 | 0.272                                                          | 0.211                                                          | 28.856  | 28.826   | 6.91e-02 |
| NP_004705 | NP_005021 | 50   | 8,158 | 0.613 | 0.163                                                          | 0.249                                                          | -34.671 | -33.500  | 5.32e-14 |
| NP_000752 | NP_000760 | 3    | 543   | 0.552 | 0.299                                                          | 0.247                                                          | 21.330  | 23.816   | 3.93e-01 |
| NP_036559 | NP_004337 | 2    | 622   | 0.322 | 0.252                                                          | 0.246                                                          | 2.153   | 3.971    | 8.75e-01 |
| NP_002825 | NP_004081 | 2    | 1,316 | 0.152 | 0.261                                                          | 0.254                                                          | 2.678   | 2.762    | 8.02e-03 |

In this table, the columns source(S) and target(T) correspond to the protein accession numbers of the corresponding bioassays of source and target tasks, respectively. The columns #cor, #act and cor% have the count of correctly classified active compounds, total number of active compounds and the percentage of correctly classified active compounds, respectively. Such compounds are denoted by the set  $\tilde{\mathcal{X}}_{B_T}^+$ . The columns  $\text{sim}(\tilde{\mathcal{X}}_{B_T}^+, \mathcal{X}_{B_S}^+)$  and  $\text{sim}(\tilde{\mathcal{X}}_{B_T}^+, \mathcal{X}_{B_T}^+)$  present the average pairwise similarities of correctly classified compounds in  $\tilde{\mathcal{X}}_{B_T}^+$  with their top-5 most similar active compounds from the source and target bioassay, respectively. The column sdiff% has the percentage difference of the average pairwise similarities from the source compounds over the target compounds. The column e-sdiff% has the average of element-wise percentage difference of similarities from the source active compounds over the target active compounds. The column p-value has the corresponding p-values for e-sdiff%.

### 3.3 Parameter Study: TAc-fc-dmpna

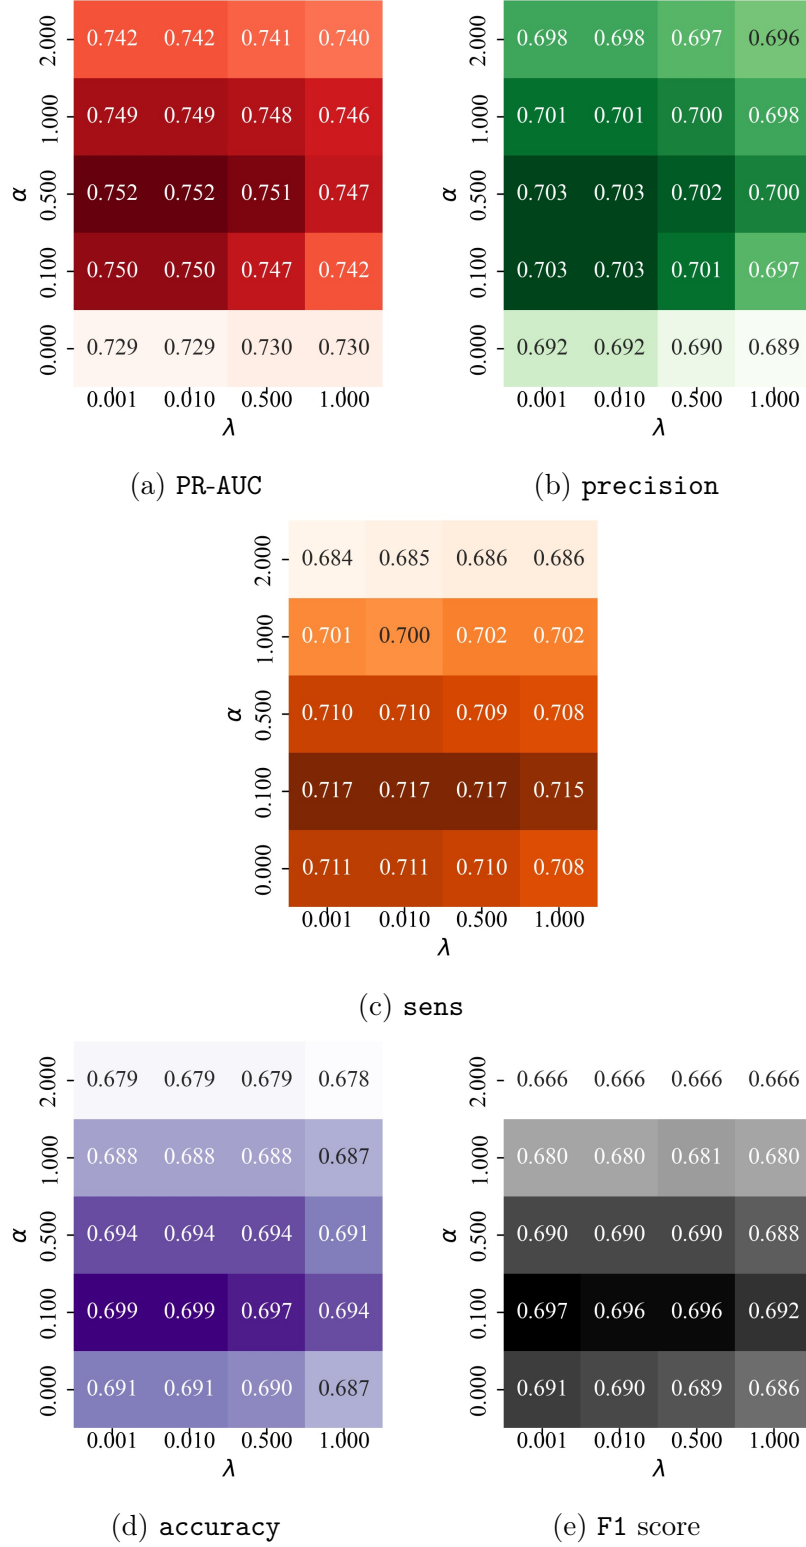

Figure S1: Parameter Study of TAc-fc-dmpna

Figure S1 presents the parameter study in **TAc-fc-dmpna** in terms of **PR-AUC**, **precision**, **sens**, **accuracy** and **F1** on  $\alpha$  (i.e., the trade-off parameter between the source and target classification losses as in Equation 4) and  $\lambda$  (i.e., the trade-off parameter between the classification and discriminator losses in Equation 13). The study was conducted over the tasks for which **TAc-dmpna** outperforms the other methods in respective metrics. The values in each cell in the figure represent the average of the best performance over the tasks with the optimal choice of other hyperparameters.

Figure S1 shows that **TAc-fc-dmpna** has the best performance in **PR-AUC** when  $\alpha = 0.5$  and  $\lambda = 0.001$  and  $0.01$ . This aligns with our observations in the parameter study for **ROC-AUC**. **TAc-fc-dmpna** has the best performance in **precision**, **sens**, **accuracy** and **F1** when  $\alpha = 0.1$  and  $\lambda = 0.001$  and  $0.01$ . Although for the metrics except **ROC-AUC** and **PR-AUC**, the best performance is achieved at a lower  $\alpha$  than  $0.5$ , optimal  $\alpha$  values are still non-zero. This provides strong evidence that the target task benefits from the transferred information from the source task. Similar to our observed trends from the parameter study for **ROC-AUC**, there is a significant performance drop for too high or too low  $\alpha$ , regardless of what  $\lambda$  is; for optimal  $\alpha$ , a  $\lambda = 0.001$  or  $0.01$  gives the best performance; for a given  $\alpha$ , higher  $\lambda$  values degrades the performance.

## 4 Compound Prioritization using dmpna

In this section, we develop a comprehensive learning-to-rank method for effective compound prioritization that jointly learns molecular graph representations via **GNN** and a scoring function  $\phi(\cdot)$  using the representations in an end-to-end manner. We denote our method as **gnnCP**. We consider the compound prioritization problem to correctly rank compounds in terms of their activities with respect to a protein target. To achieve so, **gnnCP** represents compounds using latent features that are learned from molecular graphs via a new, attention directed message passing neural network (**dmpna**) (explained in Section 4.2). We use a linear

scoring function  $\phi(\mathbf{r}_c) : \mathbb{R}^d \rightarrow \mathbb{R}$  to score the compounds as follows,

$$\phi(\mathbf{r}_c) = \mathbf{w}^\top \mathbf{r}_c, \quad (7)$$

where  $\mathbf{w}$  is a learnable parameter. Our proposed method **gnnCP** will produce a ranking of compounds induced by their predicted scores (computed using  $\phi(\mathbf{r}_c)$ ). Compounds with higher predicted scores will be ranked higher than those with lower predicted scores. Higher scores will be assigned to more active compounds in order to achieve the best ranking quality. To quantify the ranking quality, we use the popular metric non-concordance index ( $nCI$ ).  $nCI$  measures the fraction of incorrectly ranked compound pairs as follows,

$$nCI(r, \phi) = \frac{1}{|\{c_i, c_j | c_i \succ_r c_j\}|} \sum_{\{c_i, c_j | c_i \succ_r c_j\}} \mathbb{I}(c_i \preceq_\phi c_j), \quad (8)$$

where  $\mathbb{I}$  is the indicator function. In equation 8,  $c_i \succ_r c_j$  represents a pair of compounds  $c_i$  and  $c_j$  such that  $c_i$  is ranked higher than  $c_j$  in the ground truth ranking  $r$ , and  $c_i \preceq_\phi c_j$  represents that  $c_i$  is ranked lower than  $c_j$  in the predicted ranking structure induced by  $\phi$ . In essence, a lower  $nCI$  would indicate better ranking performance. Following the work,<sup>1</sup> we use  $nCI$  over the predicted ranking structure induced by  $\phi$  as our loss function  $\mathcal{L}_{rank}$ .

Since the indicator function in equation 8 is discontinuous, we use the logistic loss as a surrogate function<sup>2</sup> as follows,

$$\mathbb{I}(a \preceq b) \approx \log(1 + \exp(-(a - b))). \quad (9)$$

The loss term  $\mathcal{L}_{rank}$  for the set of compounds in a given bioassay is defined as follows,

$$\mathcal{L}_{rank} = \frac{1}{|\{c_i, c_j | c_i \succ_r c_j\}|} \sum_{\{c_i, c_j | c_i \succ_r c_j, c_i \preceq_\phi c_j\}} \log[1 + \exp(-(\mathbf{w}^\top \mathbf{z}_{c_i} - \mathbf{w}^\top \mathbf{z}_{c_j}))]. \quad (10)$$

We solve the following optimization:

$$\min_{\Theta} \mathcal{L}_{rank} + \lambda ||\Theta||_2^2, \tag{11}$$

where  $\lambda$  is the regularization parameter and  $\Theta$  is the set of trainable parameters. The above optimization encourages correct ranking of compound pairs and hence, higher scores being assigned to more active compounds.

## References

- (1) Liu, J.; Ning, X. Differential Compound Prioritization via Bidirectional Selectivity Push with Power. *Journal of Chemical Information and Modeling* **2017**, *57*, 2958–2975.
- (2) Li, H. A short introduction to learning to rank. *IEICE Transactions on Information and Systems* **2011**, *E94-D*, 1854–1862.
